# Supplementary material for: Classification of Web Phishing Kits for early detection by platform providers
Source: arXiv:2210.08273 source file (2022-10-15)
Supplement: Supplementary file 1 [file appendix_parameters.tex]

\section{Parameters}
\label{sec_appendix:parameters}
